# Supplementary material for: DocChecker: Bootstrapping Code Large Language Model for Detecting and Resolving Code-Comment Inconsistencies
Source: arXiv:2306.06347 source file (2024-02-03)
Supplement: Supplementary file 1 [file appendix.tex]

\end{table*}
